# Supplementary material for: Concept Annotation for Intelligent Textbooks
Source: arXiv:2005.11422 source file (2020-06-10)
Supplement: Supplementary file 1 [file sm_results.tex]

\begin{table}[htbp]
\begin{tabular}{|l|l|l|l|}
\hline
\textbf{Annotation Method} & \textbf{AUC} & \textbf{RMSE}  \\ \hline
Annotator 1     & 0.94               & 0.89               \\ \hline
Annotator 2     & 0.91               & 0.89               \\ \hline
Annotator 3     & 0.91               & 0.95                \\ \hline
\end{tabular}
\caption{Student modeling output on individual annotator output before discussion}
\label{smindividual}
\vspace{-1em}
\end{table}

\begin{table}[htbp]
\begin{tabular}{|l|l|l|l|}
\hline
\textbf{Annotation Method} & \textbf{AUC} & \textbf{RMSE}  \\ \hline
Annotator 1     & 0.94               & 0.89               \\ \hline
Annotator 2     & 0.91               & 0.89               \\ \hline
Annotator 3     & 0.91               & 0.95                \\ \hline
\end{tabular}
\caption{Student modeling output on combined annotation after discussion}
\label{init_sm_results}
\end{table}

\begin{table}[htbp]
\begin{tabular}{|l|l|l|l|}
\hline
\textbf{Annotation Method} & \textbf{AUC} & \textbf{RMSE}  \\ \hline
Expert     & 0.541	& 0.475     \\ \hline
IBM      & 0.624 &	0.385      \\ \hline
Gold     & 0.633	& 0.363 \\ \hline
\end{tabular}
\caption{Results of Student Performance Prediction based on baseline corpora with proposed approach}
\label{tab:smbaseline}
\end{table}
